# Supplementary material for: The 290 fixed-point sublattices of the Leech lattice
Source: arXiv:1505.06420 ancillary file (2016-01-13)
Supplement: Supplementary file 1 [file supptable2-jalg.pdf]

Supplementary Table 2: Gram matrices of the fixed-point lattices.

$$\#1 \quad \begin{pmatrix}
8 & 4 & 4 & 4 & 4 & 4 & 4 & 2 & 4 & 4 & 4 & 2 & 4 & 2 & 2 & 2 & 4 & 2 & 2 & 2 & 0 & 0 & 0 & -3 \\
4 & 4 & 2 & 2 & 2 & 2 & 2 & 2 & 2 & 2 & 2 & 2 & 2 & 2 & 1 & 1 & 2 & 1 & 1 & 2 & 1 & 0 & 0 & -1 \\
4 & 2 & 4 & 2 & 2 & 2 & 2 & 2 & 2 & 2 & 2 & 2 & 2 & 1 & 2 & 1 & 2 & 2 & 1 & 1 & 1 & 0 & 0 & -1 \\
4 & 2 & 2 & 4 & 2 & 2 & 2 & 2 & 2 & 2 & 2 & 2 & 2 & 1 & 1 & 2 & 2 & 1 & 2 & 1 & 1 & 0 & 0 & -1 \\
4 & 2 & 2 & 2 & 4 & 2 & 2 & 2 & 2 & 2 & 2 & 1 & 2 & 2 & 2 & 2 & 2 & 2 & 2 & 2 & 1 & 0 & 0 & -1 \\
4 & 2 & 2 & 2 & 2 & 4 & 2 & 2 & 2 & 2 & 2 & 1 & 2 & 2 & 1 & 1 & 2 & 1 & 2 & 1 & 0 & 0 & 0 & -1 \\
4 & 2 & 2 & 2 & 2 & 2 & 4 & 2 & 2 & 2 & 2 & 1 & 2 & 1 & 2 & 1 & 2 & 1 & 1 & 2 & 0 & 0 & 0 & -1 \\
2 & 2 & 2 & 2 & 2 & 2 & 2 & 4 & 1 & 1 & 1 & 2 & 1 & 2 & 2 & 2 & 1 & 2 & 2 & 2 & 2 & 0 & 0 & 1 \\
4 & 2 & 2 & 2 & 2 & 2 & 2 & 1 & 4 & 2 & 2 & 2 & 2 & 2 & 2 & 2 & 2 & 2 & 2 & 2 & 1 & 1 & 1 & -1 \\
4 & 2 & 2 & 2 & 2 & 2 & 2 & 1 & 2 & 4 & 2 & 2 & 2 & 2 & 1 & 1 & 2 & 2 & 1 & 1 & 0 & 1 & 0 & -1 \\
4 & 2 & 2 & 2 & 2 & 2 & 2 & 1 & 2 & 2 & 4 & 2 & 2 & 1 & 2 & 1 & 2 & 1 & 2 & 1 & 0 & 0 & 1 & -1 \\
2 & 2 & 2 & 2 & 1 & 1 & 1 & 2 & 2 & 2 & 2 & 4 & 1 & 2 & 2 & 2 & 1 & 2 & 2 & 2 & 2 & 1 & 1 & 1 \\
4 & 2 & 2 & 2 & 2 & 2 & 2 & 1 & 2 & 2 & 2 & 1 & 4 & 2 & 2 & 2 & 2 & 1 & 1 & 1 & 1 & 1 & 1 & -1 \\
2 & 2 & 1 & 1 & 2 & 2 & 1 & 2 & 2 & 2 & 1 & 2 & 2 & 4 & 2 & 2 & 1 & 2 & 2 & 2 & 2 & 2 & 1 & 1 \\
2 & 1 & 2 & 1 & 2 & 1 & 2 & 2 & 2 & 1 & 2 & 2 & 2 & 2 & 4 & 2 & 1 & 2 & 2 & 2 & 2 & 1 & 2 & 1 \\
2 & 1 & 1 & 2 & 2 & 1 & 1 & 2 & 2 & 1 & 1 & 2 & 2 & 2 & 2 & 4 & 1 & 2 & 2 & 2 & 2 & 1 & 1 & 1 \\
4 & 2 & 2 & 2 & 2 & 2 & 2 & 1 & 2 & 2 & 2 & 1 & 2 & 1 & 1 & 1 & 4 & 2 & 2 & 2 & 1 & 1 & 1 & -1 \\
2 & 1 & 2 & 1 & 2 & 1 & 1 & 2 & 2 & 2 & 1 & 2 & 1 & 2 & 2 & 2 & 2 & 4 & 2 & 2 & 2 & 2 & 1 & 1 \\
2 & 1 & 1 & 2 & 2 & 2 & 1 & 2 & 2 & 1 & 2 & 2 & 1 & 2 & 2 & 2 & 2 & 2 & 4 & 2 & 2 & 1 & 2 & 1 \\
2 & 2 & 1 & 1 & 2 & 1 & 2 & 2 & 2 & 1 & 1 & 2 & 1 & 2 & 2 & 2 & 2 & 2 & 2 & 4 & 2 & 1 & 1 & 1 \\
0 & 1 & 1 & 1 & 1 & 0 & 0 & 2 & 1 & 0 & 0 & 2 & 1 & 2 & 2 & 2 & 1 & 2 & 2 & 2 & 4 & 2 & 2 & 2 \\
0 & 0 & 0 & 0 & 0 & 0 & 0 & 0 & 1 & 1 & 0 & 1 & 1 & 2 & 1 & 1 & 1 & 2 & 1 & 1 & 2 & 4 & 2 & 2 \\
0 & 0 & 0 & 0 & 0 & 0 & 0 & 0 & 1 & 0 & 1 & 1 & 1 & 1 & 2 & 1 & 1 & 1 & 2 & 1 & 2 & 2 & 4 & 2 \\
-3 & -1 & -1 & -1 & -1 & -1 & -1 & 1 & -1 & -1 & -1 & 1 & -1 & 1 & 1 & 1 & -1 & 1 & 1 & 1 & 2 & 2 & 2 & 4
\end{pmatrix},$$

$$\#2 \quad \begin{pmatrix}
4 & -1 & -2 & -2 & -1 & -1 & -2 & -2 & 2 & 2 & -2 & -1 & -1 & 1 & -2 & 2 \\
-1 & 4 & 2 & -1 & 2 & -1 & 2 & 2 & 0 & -1 & -1 & 2 & 2 & 1 & -1 & 1 \\
-2 & 2 & 4 & 1 & 1 & 1 & 1 & 2 & -2 & -2 & 0 & 2 & 0 & 0 & 1 & -1 \\
-2 & -1 & 1 & 4 & -1 & 2 & 1 & 1 & -1 & -2 & 1 & 0 & 0 & 0 & 1 & -1 \\
-1 & 2 & 1 & -1 & 4 & -2 & 2 & 0 & -1 & -1 & -1 & 2 & 0 & -1 & 0 & -1 \\
-1 & -1 & 1 & 2 & -2 & 4 & -1 & 0 & -1 & -1 & 1 & 0 & -1 & 1 & 0 & 0 \\
-2 & 2 & 1 & 1 & 2 & -1 & 4 & 2 & 0 & -2 & 0 & 1 & 2 & 0 & 1 & 0 \\
-2 & 2 & 2 & 1 & 0 & 0 & 2 & 4 & -1 & -2 & 0 & 0 & 2 & 1 & 1 & 0 \\
2 & 0 & -2 & -1 & -1 & -1 & 0 & -1 & 4 & 2 & -1 & 0 & 1 & 0 & -2 & 2 \\
2 & -1 & -2 & -2 & -1 & -1 & -2 & -2 & 2 & 4 & 0 & 0 & -1 & 0 & -1 & 0 \\
-2 & -1 & 0 & 1 & -1 & 1 & 0 & 0 & -1 & 0 & 4 & 0 & 1 & -1 & 2 & -2 \\
-1 & 2 & 2 & 0 & 2 & 0 & 1 & 0 & 0 & 0 & 0 & 4 & 0 & 0 & -1 & -1 \\
-1 & 2 & 0 & 0 & 0 & -1 & 2 & 2 & 1 & -1 & 1 & 0 & 4 & 0 & 0 & 1 \\
1 & 1 & 0 & 0 & -1 & 1 & 0 & 1 & 0 & 0 & -1 & 0 & 0 & 4 & -1 & 2 \\
-2 & -1 & 1 & 1 & 0 & 0 & 1 & 1 & -2 & -1 & 2 & -1 & 0 & -1 & 4 & -2 \\
2 & 1 & -1 & -1 & -1 & 0 & 0 & 0 & 2 & 0 & -2 & -1 & 1 & 2 & -2 & 4
\end{pmatrix},$$

$$\#3 \quad \begin{pmatrix}
4 & -2 & 0 & 1 & 2 & -1 & -2 & 2 & 0 & -1 & -1 & 2 \\
-2 & 4 & 0 & -1 & 0 & -1 & 0 & -2 & 0 & -1 & -1 & 0 \\
0 & 0 & 4 & 1 & 0 & 2 & -1 & 1 & -2 & -2 & -2 & 2 \\
1 & -1 & 1 & 4 & -1 & 0 & 1 & 0 & 1 & -2 & 0 & 0 \\
2 & 0 & 0 & -1 & 4 & 0 & -1 & 1 & 0 & 0 & -2 & 2 \\
-1 & -1 & 2 & 0 & 0 & 4 & 1 & 0 & -1 & 0 & 0 & 0 \\
-2 & 0 & -1 & 1 & -1 & 1 & 4 & -2 & 2 & 1 & 1 & -2 \\
2 & -2 & 1 & 0 & 1 & 0 & -2 & 4 & -2 & 0 & 0 & 2 \\
0 & 0 & -2 & 1 & 0 & -1 & 2 & -2 & 4 & 1 & 1 & -2 \\
-1 & -1 & -2 & -2 & 0 & 0 & 1 & 0 & 1 & 4 & 2 & -2 \\
-1 & -1 & -2 & 0 & -2 & 0 & 1 & 0 & 1 & 2 & 4 & -2 \\
2 & 0 & 2 & 0 & 2 & 0 & -2 & 2 & -2 & -2 & -2 & 4
\end{pmatrix}, \quad \#4 \quad \begin{pmatrix}
4 & 1 & -2 & -2 & 1 & 2 & -2 & -1 & -2 & -2 & -2 & 2 \\
1 & 4 & -2 & -1 & 1 & 0 & 0 & 1 & -2 & 1 & 1 & 2 \\
-2 & -2 & 4 & 2 & -2 & 0 & 0 & 1 & 1 & 1 & 1 & -1 \\
-2 & -1 & 2 & 4 & 0 & -2 & 1 & 2 & 0 & 2 & 0 & -2 \\
1 & 1 & -2 & 0 & 4 & -1 & -1 & -1 & -1 & 1 & 0 & -1 \\
2 & 0 & 0 & -2 & -1 & 4 & -2 & 0 & 0 & -1 & 0 & 2 \\
-2 & 0 & 0 & 1 & -1 & -2 & 4 & 1 & 0 & 0 & 1 & 0 \\
-1 & 1 & 1 & 2 & -1 & 0 & 1 & 4 & 0 & 2 & 1 & 0 \\
-2 & -2 & 1 & 0 & -1 & 0 & 0 & 0 & 4 & 0 & 0 & -2 \\
-2 & 1 & 1 & 2 & 1 & -1 & 0 & 2 & 0 & 4 & 2 & -1 \\
-2 & 1 & 1 & 0 & 0 & 0 & 1 & 1 & 0 & 2 & 4 & 0 \\
2 & 2 & -1 & -2 & -1 & 2 & 0 & 0 & -2 & -1 & 0 & 4
\end{pmatrix},$$

$$\#5 \quad \begin{pmatrix}
4 & -2 & 0 & -2 & 0 & 2 & -2 & 0 & 0 & 0 & 2 & -2 \\
-2 & 6 & -2 & 2 & 2 & -2 & 2 & -2 & 2 & -2 & -2 & 2 \\
0 & -2 & 4 & -2 & -2 & 2 & 0 & 2 & -2 & 2 & 0 & 0 \\
-2 & 2 & -2 & 4 & 2 & -2 & 2 & 0 & 0 & 0 & -2 & 2 \\
0 & 2 & -2 & 2 & 4 & 0 & 0 & 0 & 0 & 0 & 0 & 0 \\
2 & -2 & 2 & -2 & 0 & 4 & -2 & 2 & -2 & 2 & 2 & -2 \\
-2 & 2 & 0 & 2 & 0 & -2 & 4 & 0 & 0 & 0 & -2 & 2 \\
0 & -2 & 2 & 0 & 0 & 2 & 0 & 4 & -2 & 2 & 0 & 0 \\
0 & 2 & -2 & 0 & 0 & -2 & 0 & -2 & 4 & -2 & 0 & 0 \\
0 & -2 & 2 & 0 & 0 & 2 & 0 & 2 & -2 & 4 & 0 & 0 \\
2 & -2 & 0 & -2 & 0 & 2 & -2 & 0 & 0 & 0 & 4 & -2 \\
-2 & 2 & 0 & 2 & 0 & -2 & 2 & 0 & 0 & 0 & -2 & 4
\end{pmatrix}, \quad \#6 \quad \begin{pmatrix}
4 & -2 & -2 & -2 & -2 & -2 & -2 & -2 & -2 & 2 \\
-2 & 4 & 0 & 1 & 1 & 2 & 2 & 2 & 0 & 0 \\
-2 & 0 & 4 & 2 & 0 & 0 & 2 & 0 & 2 & -2 \\
-2 & 1 & 2 & 4 & 0 & 2 & 1 & 2 & 0 & -1 \\
-2 & 1 & 0 & 0 & 4 & 0 & 1 & 2 & 2 & -1 \\
-2 & 2 & 0 & 2 & 0 & 4 & 0 & 2 & 0 & 0 \\
-2 & 2 & 2 & 1 & 1 & 0 & 4 & 0 & 2 & -2 \\
-2 & 2 & 0 & 2 & 2 & 2 & 0 & 4 & 0 & 0 \\
-2 & 0 & 2 & 0 & 2 & 0 & 2 & 0 & 4 & -2 \\
2 & 0 & -2 & -1 & -1 & 0 & -2 & 0 & -2 & 4
\end{pmatrix},$$

$$\#7\ \begin{pmatrix} 4 & -2 & -2 & -1 & 2 & -1 & -2 & -2 & -2 & -1 \\ -2 & 4 & 0 & 2 & -1 & -1 & 1 & 2 & 2 & -1 \\ -2 & 0 & 4 & 1 & -2 & 2 & 2 & 1 & 2 & 2 \\ -1 & 2 & 1 & 4 & -2 & -1 & 0 & 0 & 1 & 1 \\ 2 & -1 & -2 & -2 & 4 & -1 & 0 & 0 & -2 & -2 \\ -1 & -1 & 2 & -1 & -1 & 4 & 2 & 1 & 0 & 2 \\ -2 & 1 & 2 & 0 & 0 & 2 & 4 & 2 & 1 & 0 \\ -2 & 2 & 1 & 0 & 0 & 1 & 2 & 4 & 2 & -1 \\ -2 & 2 & 2 & 1 & -2 & 0 & 1 & 2 & 4 & 0 \\ -1 & -1 & 2 & 1 & -2 & 2 & 0 & -1 & 0 & 4 \end{pmatrix},\ \#8\ \begin{pmatrix} 4 & -2 & -2 & 2 & 2 & 2 & -2 & -2 & 2 & -2 \\ -2 & 4 & 0 & 0 & -2 & 0 & 2 & 2 & -2 & 0 \\ -2 & 0 & 4 & -2 & -2 & -2 & 0 & 0 & 0 & 2 \\ 2 & 0 & -2 & 4 & 2 & 2 & 0 & 0 & 0 & -2 \\ 2 & -2 & -2 & 2 & 4 & 2 & 0 & 0 & 0 & -2 \\ 2 & 0 & -2 & 2 & 2 & 4 & 0 & 0 & 0 & -2 \\ -2 & 2 & 0 & 0 & 0 & 0 & 4 & 2 & -2 & 0 \\ -2 & 2 & 0 & 0 & 0 & 0 & 2 & 4 & -2 & 0 \\ 2 & -2 & 0 & 0 & 0 & 0 & -2 & -2 & 4 & 0 \\ -2 & 0 & 2 & -2 & -2 & -2 & 0 & 0 & 0 & 4 \end{pmatrix},$$

$$\#9\ \begin{pmatrix} 4 & 1 & -1 & -1 & 1 & 2 & -2 & -2 & -1 & -2 \\ 1 & 4 & 1 & -2 & -1 & 2 & -2 & -2 & -2 & -1 \\ -1 & 1 & 4 & 1 & 1 & -1 & 0 & 0 & -2 & 2 \\ -1 & -2 & 1 & 4 & 0 & -1 & 2 & 0 & 1 & 2 \\ 1 & -1 & 1 & 0 & 4 & 0 & -1 & 1 & -1 & 1 \\ 2 & 2 & -1 & -1 & 0 & 4 & -1 & -1 & 0 & -2 \\ -2 & -2 & 0 & 2 & -1 & -1 & 4 & 2 & 1 & 1 \\ -2 & -2 & 0 & 0 & 1 & -1 & 2 & 4 & 1 & 1 \\ -1 & -2 & -2 & 1 & -1 & 0 & 1 & 1 & 4 & -1 \\ -2 & -1 & 2 & 2 & 1 & -2 & 1 & 1 & -1 & 4 \end{pmatrix},\quad \#10\ \begin{pmatrix} 4 & -2 & -2 & -2 & 2 & 2 & -2 & -2 & -2 \\ -2 & 4 & 1 & 2 & 0 & -2 & 0 & 0 & 0 \\ -2 & 1 & 4 & 0 & -2 & -2 & 0 & 0 & 0 \\ -2 & 2 & 0 & 4 & 0 & 0 & 2 & 2 & 2 \\ 2 & 0 & -2 & 0 & 4 & 0 & 0 & 0 & 0 \\ 2 & -2 & -2 & 0 & 0 & 4 & 0 & 0 & 0 \\ -2 & 0 & 0 & 2 & 0 & 0 & 4 & 2 & 2 \\ -2 & 0 & 0 & 2 & 0 & 0 & 2 & 4 & 2 \\ -2 & 0 & 0 & 2 & 0 & 0 & 2 & 2 & 4 \end{pmatrix},$$

$$\#11\ \begin{pmatrix} 4 & 2 & 2 & -2 & -2 & -2 & -2 & -2 & 0 \\ 2 & 4 & 2 & -2 & -2 & -2 & 0 & -2 & 0 \\ 2 & 2 & 4 & -2 & 0 & 0 & -2 & 0 & 0 \\ -2 & -2 & -2 & 4 & 2 & 2 & 0 & 0 & 0 \\ -2 & -2 & 0 & 2 & 4 & 2 & 0 & 2 & 0 \\ -2 & -2 & 0 & 2 & 2 & 4 & 0 & 2 & 0 \\ -2 & 0 & -2 & 0 & 0 & 0 & 4 & 0 & 0 \\ -2 & -2 & 0 & 0 & 2 & 2 & 0 & 4 & 0 \\ 0 & 0 & 0 & 0 & 0 & 0 & 0 & 0 & 4 \end{pmatrix},\quad \#12\ \begin{pmatrix} 4 & 2 & 2 & -2 & -2 & -2 & 2 & -2 & 2 \\ 2 & 4 & 2 & -2 & -2 & -2 & 2 & -2 & 2 \\ 2 & 2 & 4 & -2 & 0 & -2 & 2 & -2 & 2 \\ -2 & -2 & -2 & 4 & 0 & 2 & -2 & 2 & -2 \\ -2 & -2 & 0 & 0 & 4 & 0 & 0 & 0 & 0 \\ -2 & -2 & -2 & 2 & 0 & 4 & -2 & 2 & -2 \\ 2 & 2 & 2 & -2 & 0 & -2 & 4 & -2 & 2 \\ -2 & -2 & -2 & 2 & 0 & 2 & -2 & 4 & -2 \\ 2 & 2 & 2 & -2 & 0 & -2 & 2 & -2 & 4 \end{pmatrix},$$

$$\#13\ \begin{pmatrix} 4 & -2 & -2 & 2 & -1 & -2 & 1 & -1 & -2 \\ -2 & 4 & 0 & -2 & 2 & 0 & -2 & 2 & 2 \\ -2 & 0 & 4 & -1 & 1 & 2 & 1 & -1 & 2 \\ 2 & -2 & -1 & 4 & -2 & -2 & 2 & -2 & -2 \\ -1 & 2 & 1 & -2 & 4 & 0 & 0 & 2 & 1 \\ -2 & 0 & 2 & -2 & 0 & 4 & 0 & 0 & 2 \\ 1 & -2 & 1 & 2 & 0 & 0 & 4 & -2 & -1 \\ -1 & 2 & -1 & -2 & 2 & 0 & -2 & 4 & 1 \\ -2 & 2 & 2 & -2 & 1 & 2 & -1 & 1 & 4 \end{pmatrix},\quad \#14\ \begin{pmatrix} 4 & -2 & -2 & 2 & -2 & -2 & 2 & -2 \\ -2 & 4 & 2 & -2 & 2 & 2 & -2 & 0 \\ -2 & 2 & 4 & -2 & 0 & 0 & 0 & 2 \\ 2 & -2 & -2 & 4 & -2 & 0 & 0 & -2 \\ -2 & 2 & 0 & -2 & 4 & 2 & -2 & 0 \\ -2 & 2 & 0 & 0 & 2 & 4 & -2 & 0 \\ 2 & -2 & 0 & 0 & -2 & -2 & 4 & 0 \\ -2 & 0 & 2 & -2 & 0 & 0 & 0 & 4 \end{pmatrix},$$

$$\#15\ \begin{pmatrix} 4 & -2 & -2 & -1 & -1 & 2 & 1 & -2 \\ -2 & 4 & 2 & 2 & -1 & -1 & 1 & 0 \\ -2 & 2 & 4 & 2 & -1 & 0 & 1 & 1 \\ -1 & 2 & 2 & 4 & -2 & 1 & 2 & -1 \\ -1 & -1 & -1 & -2 & 4 & -2 & -1 & 2 \\ 2 & -1 & 0 & 1 & -2 & 4 & 2 & -2 \\ 1 & 1 & 1 & 2 & -1 & 2 & 4 & -2 \\ -2 & 0 & 1 & -1 & 2 & -2 & -2 & 4 \end{pmatrix},\quad \#16\ \begin{pmatrix} 4 & -2 & -2 & -2 & -2 & -2 & 2 & -2 \\ -2 & 4 & 2 & 2 & 2 & 2 & -2 & 2 \\ -2 & 2 & 4 & 2 & 0 & 2 & -2 & 2 \\ -2 & 2 & 2 & 4 & 2 & 2 & -2 & 2 \\ -2 & 2 & 0 & 2 & 4 & 2 & -2 & 2 \\ -2 & 2 & 2 & 2 & 2 & 4 & -2 & 2 \\ 2 & -2 & -2 & -2 & -2 & -2 & 4 & -2 \\ -2 & 2 & 2 & 2 & 2 & 2 & -2 & 4 \end{pmatrix},$$

$$\#17\ \begin{pmatrix} 4 & -2 & 2 & -2 & -2 & -2 & 1 & -1 \\ -2 & 4 & -2 & 2 & 0 & 0 & -2 & 2 \\ 2 & -2 & 4 & -2 & -2 & 0 & 1 & -1 \\ -2 & 2 & -2 & 4 & 0 & 0 & 0 & 2 \\ -2 & 0 & -2 & 0 & 4 & 2 & 0 & 0 \\ -2 & 0 & 0 & 0 & 2 & 4 & -1 & -1 \\ 1 & -2 & 1 & 0 & 0 & -1 & 4 & 0 \\ -1 & 2 & -1 & 2 & 0 & -1 & 0 & 4 \end{pmatrix},\quad \#18\ \begin{pmatrix} 4 & -2 & 2 & 1 & 1 & 1 & 2 & -1 \\ -2 & 4 & -2 & 0 & 0 & -1 & -2 & -1 \\ 2 & -2 & 4 & 1 & -1 & 2 & 0 & 0 \\ 1 & 0 & 1 & 4 & 0 & 2 & -1 & 1 \\ 1 & 0 & -1 & 0 & 4 & 1 & 1 & -2 \\ 1 & -1 & 2 & 2 & 1 & 4 & 0 & 0 \\ 2 & -2 & 0 & -1 & 1 & 0 & 4 & 0 \\ -1 & -1 & 0 & 1 & -2 & 0 & 0 & 4 \end{pmatrix},$$

$$\#19\ \begin{pmatrix} 4 & -1 & -1 & -2 & 1 & -2 & 2 & -2 \\ -1 & 4 & 2 & 1 & -2 & -1 & 1 & 2 \\ -1 & 2 & 4 & 2 & -2 & 1 & -1 & 0 \\ -2 & 1 & 2 & 4 & -2 & 1 & -1 & 1 \\ 1 & -2 & -2 & -2 & 4 & 1 & 1 & 0 \\ -2 & -1 & 1 & 1 & 1 & 4 & -2 & 0 \\ 2 & 1 & -1 & -1 & 1 & -2 & 4 & 0 \\ -2 & 2 & 0 & 1 & 0 & 0 & 0 & 4 \end{pmatrix},\quad \#20\ \begin{pmatrix} 4 & -2 & 2 & 1 & 2 & 2 & 1 & -2 \\ -2 & 4 & -2 & -2 & -1 & -2 & 1 & 2 \\ 2 & -2 & 4 & 2 & 2 & 1 & -1 & -2 \\ 1 & -2 & 2 & 4 & 1 & 2 & -2 & 0 \\ 2 & -1 & 2 & 1 & 4 & 2 & -1 & 0 \\ 2 & -2 & 1 & 2 & 2 & 4 & 0 & 0 \\ 1 & 1 & -1 & -2 & -1 & 0 & 4 & -1 \\ -2 & 2 & -2 & 0 & 0 & 0 & -1 & 4 \end{pmatrix},$$

$$\#21\ \begin{pmatrix} 4 & -2 & -2 & -2 & 0 & 0 & 0 & 0 \\ -2 & 4 & 0 & 2 & 0 & 0 & 0 & 0 \\ -2 & 0 & 4 & 2 & 0 & 0 & 0 & 0 \\ -2 & 2 & 2 & 4 & 0 & 0 & 0 & 0 \\ 0 & 0 & 0 & 0 & 4 & -2 & 2 & 2 \\ 0 & 0 & 0 & 0 & -2 & 4 & -2 & 0 \\ 0 & 0 & 0 & 0 & 2 & -2 & 4 & 2 \\ 0 & 0 & 0 & 0 & 2 & 0 & 2 & 4 \end{pmatrix},\quad \#22\ \begin{pmatrix} 6 & -3 & 3 & -3 & -3 & 3 & -3 & -3 \\ -3 & 6 & -3 & 0 & 3 & -3 & 0 & 0 \\ 3 & -3 & 6 & 0 & 0 & 0 & -3 & -3 \\ -3 & 0 & 0 & 6 & 3 & 0 & 3 & 3 \\ -3 & 3 & 0 & 3 & 6 & -3 & 0 & 0 \\ 3 & -3 & 0 & 0 & -3 & 6 & 0 & 0 \\ -3 & 0 & -3 & 3 & 0 & 0 & 6 & 3 \\ -3 & 0 & -3 & 3 & 0 & 0 & 3 & 6 \end{pmatrix},$$

$$\#23\quad \begin{pmatrix} 4 & 2 & 0 & 0 & 0 & 0 & 0 & 0 \\ 2 & 6 & 2 & 2 & -2 & -2 & 2 & 2 \\ 0 & 2 & 4 & 0 & 0 & 0 & 0 & 0 \\ 0 & 2 & 0 & 4 & -2 & -2 & 0 & 0 \\ 0 & -2 & 0 & -2 & 4 & 2 & -2 & 0 \\ 0 & -2 & 0 & -2 & 2 & 4 & -2 & 0 \\ 0 & 2 & 0 & 0 & -2 & -2 & 4 & 0 \\ 0 & 2 & 0 & 0 & 0 & 0 & 0 & 4 \end{pmatrix}, \qquad \#24\quad \begin{pmatrix} 4 & 2 & -2 & -2 & 2 & -2 & -2 \\ 2 & 4 & -2 & 0 & 2 & -1 & -2 \\ -2 & -2 & 4 & 0 & 0 & 0 & 2 \\ -2 & 0 & 0 & 4 & -2 & 2 & 0 \\ 2 & 2 & 0 & -2 & 4 & -1 & 0 \\ -2 & -1 & 0 & 2 & -1 & 4 & 0 \\ -2 & -2 & 2 & 0 & 0 & 0 & 4 \end{pmatrix},$$

$$\#25\quad \begin{pmatrix} 4 & -2 & -2 & -2 & 2 & 2 & -2 \\ -2 & 4 & 2 & 0 & -2 & 0 & 0 \\ -2 & 2 & 4 & 0 & 0 & 0 & 0 \\ -2 & 0 & 0 & 4 & -2 & -2 & 2 \\ 2 & -2 & 0 & -2 & 4 & 2 & -2 \\ 2 & 0 & 0 & -2 & 2 & 4 & -2 \\ -2 & 0 & 0 & 2 & -2 & -2 & 4 \end{pmatrix}, \qquad \#26\quad \begin{pmatrix} 4 & -2 & -2 & -2 & -2 & 2 & 2 \\ -2 & 4 & 2 & 0 & 1 & 0 & 0 \\ -2 & 2 & 4 & 2 & 1 & -2 & -2 \\ -2 & 0 & 2 & 4 & 0 & -2 & -2 \\ -2 & 1 & 1 & 0 & 4 & 0 & -1 \\ 2 & 0 & -2 & -2 & 0 & 4 & 2 \\ 2 & 0 & -2 & -2 & -1 & 2 & 4 \end{pmatrix},$$

$$\#27\quad \begin{pmatrix} 4 & 2 & -2 & 2 & -2 & 2 & 0 \\ 2 & 4 & -2 & 2 & 0 & 0 & 0 \\ -2 & -2 & 4 & -2 & 2 & 0 & 0 \\ 2 & 2 & -2 & 4 & 0 & 0 & 0 \\ -2 & 0 & 2 & 0 & 4 & -2 & 0 \\ 2 & 0 & 0 & 0 & -2 & 4 & 0 \\ 0 & 0 & 0 & 0 & 0 & 0 & 4 \end{pmatrix}, \qquad \#28\quad \begin{pmatrix} 4 & 1 & -2 & -1 & -1 & -2 & -2 \\ 1 & 4 & 1 & -2 & -2 & 0 & 0 \\ -2 & 1 & 4 & -1 & -1 & 2 & 2 \\ -1 & -2 & -1 & 4 & 0 & 0 & 0 \\ -1 & -2 & -1 & 0 & 4 & 0 & 0 \\ -2 & 0 & 2 & 0 & 0 & 4 & 0 \\ -2 & 0 & 2 & 0 & 0 & 0 & 4 \end{pmatrix},$$

$$\#29\quad \begin{pmatrix} 4 & -2 & -2 & 1 & -2 & 1 & -2 \\ -2 & 4 & 2 & -1 & 2 & 1 & 2 \\ -2 & 2 & 4 & -2 & 1 & 1 & 0 \\ 1 & -1 & -2 & 4 & -2 & 1 & 0 \\ -2 & 2 & 1 & -2 & 4 & -1 & 1 \\ 1 & 1 & 1 & 1 & -1 & 4 & -1 \\ -2 & 2 & 0 & 0 & 1 & -1 & 4 \end{pmatrix}, \qquad \#30\quad \begin{pmatrix} 4 & -2 & 0 & 0 & 0 & 0 & 0 \\ -2 & 6 & -2 & 2 & -2 & 2 & -2 \\ 0 & -2 & 4 & 0 & 0 & 0 & 0 \\ 0 & 2 & 0 & 4 & 0 & 0 & 0 \\ 0 & -2 & 0 & 0 & 4 & 0 & 2 \\ 0 & 2 & 0 & 0 & 0 & 4 & 0 \\ 0 & -2 & 0 & 0 & 2 & 0 & 4 \end{pmatrix},$$

$$\#31\quad \begin{pmatrix} 4 & 1 & -2 & -2 & -2 & 1 & -1 \\ 1 & 4 & 1 & 1 & 0 & 2 & -1 \\ -2 & 1 & 4 & 2 & 0 & -1 & -1 \\ -2 & 1 & 2 & 4 & 0 & -1 & -1 \\ -2 & 0 & 0 & 0 & 4 & 0 & 2 \\ 1 & 2 & -1 & -1 & 0 & 4 & 1 \\ -1 & -1 & -1 & -1 & 2 & 1 & 4 \end{pmatrix}, \qquad \#32\quad \begin{pmatrix} 4 & -2 & -2 & 2 & 0 & 0 & 0 \\ -2 & 4 & 0 & -2 & 0 & 0 & 0 \\ -2 & 0 & 4 & -2 & 0 & 0 & 0 \\ 2 & -2 & -2 & 4 & 0 & 0 & 0 \\ 0 & 0 & 0 & 0 & 4 & 0 & 0 \\ 0 & 0 & 0 & 0 & 0 & 4 & 0 \\ 0 & 0 & 0 & 0 & 0 & 0 & 4 \end{pmatrix},$$

$$\#33\quad \begin{pmatrix} 4 & -2 & 2 & 2 & -2 & 2 \\ -2 & 4 & -2 & 0 & 0 & -2 \\ 2 & -2 & 4 & 2 & 0 & 0 \\ 2 & 0 & 2 & 4 & -2 & 0 \\ -2 & 0 & 0 & -2 & 4 & -2 \\ 2 & -2 & 0 & 0 & -2 & 4 \end{pmatrix}, \qquad \#34\quad \begin{pmatrix} 4 & -2 & -2 & -2 & 2 & -2 \\ -2 & 4 & 2 & 2 & 0 & 2 \\ -2 & 2 & 4 & 2 & -2 & 2 \\ -2 & 2 & 2 & 4 & -2 & 2 \\ 2 & 0 & -2 & -2 & 4 & -2 \\ -2 & 2 & 2 & 2 & -2 & 4 \end{pmatrix},$$

$$\#35\quad \begin{pmatrix} 4 & -1 & -2 & 2 & 2 & -2 \\ -1 & 4 & 2 & 1 & -2 & 2 \\ -2 & 2 & 4 & -1 & -1 & 1 \\ 2 & 1 & -1 & 4 & 1 & -1 \\ 2 & -2 & -1 & 1 & 4 & -1 \\ -2 & 2 & 1 & -1 & -1 & 4 \end{pmatrix}, \qquad \#36\quad \begin{pmatrix} 4 & -2 & -2 & -2 & 2 & 2 \\ -2 & 4 & 0 & 0 & -2 & 0 \\ -2 & 0 & 4 & 2 & -2 & -2 \\ -2 & 0 & 2 & 4 & 0 & -2 \\ 2 & -2 & -2 & 0 & 4 & 0 \\ 2 & 0 & -2 & -2 & 0 & 4 \end{pmatrix},$$

$$\#37\quad \begin{pmatrix} 4 & -1 & 2 & -2 & -2 & 1 \\ -1 & 4 & 1 & 2 & 2 & -2 \\ 2 & 1 & 4 & 0 & 0 & 1 \\ -2 & 2 & 0 & 4 & 2 & 0 \\ -2 & 2 & 0 & 2 & 4 & -2 \\ 1 & -2 & 1 & 0 & -2 & 4 \end{pmatrix}, \qquad \#38\quad \begin{pmatrix} 4 & -1 & 1 & -2 & -2 & -2 \\ -1 & 4 & -2 & -1 & -1 & 0 \\ 1 & -2 & 4 & -1 & 1 & 0 \\ -2 & -1 & -1 & 4 & 2 & 2 \\ -2 & -1 & 1 & 2 & 4 & 2 \\ -2 & 0 & 0 & 2 & 2 & 4 \end{pmatrix},$$

$$\#39\quad \begin{pmatrix} 4 & 2 & 0 & -1 & -1 & -2 \\ 2 & 4 & 1 & 1 & -2 & -2 \\ 0 & 1 & 4 & -1 & -2 & 1 \\ -1 & 1 & -1 & 4 & 1 & 0 \\ -1 & -2 & -2 & 1 & 4 & 1 \\ -2 & -2 & 1 & 0 & 1 & 4 \end{pmatrix}, \quad \#40\quad \begin{pmatrix} 4 & -2 & -2 & 2 & 0 & 0 \\ -2 & 4 & 0 & -2 & 0 & 0 \\ -2 & 0 & 4 & -2 & 0 & 0 \\ 2 & -2 & -2 & 4 & 0 & 0 \\ 0 & 0 & 0 & 0 & 4 & 0 \\ 0 & 0 & 0 & 0 & 0 & 4 \end{pmatrix}, \quad \#41\quad \begin{pmatrix} 4 & -2 & 0 & 0 & 0 & 0 \\ -2 & 6 & 2 & 2 & 2 & 2 \\ 0 & 2 & 4 & 0 & 0 & 0 \\ 0 & 2 & 0 & 4 & 0 & 0 \\ 0 & 2 & 0 & 0 & 4 & 0 \\ 0 & 2 & 0 & 0 & 0 & 4 \end{pmatrix},$$

$$\#42\quad \begin{pmatrix} 4 & -2 & -2 & -2 & -2 & 0 \\ -2 & 4 & 0 & 2 & 2 & 0 \\ -2 & 0 & 4 & 2 & 0 & 0 \\ -2 & 2 & 2 & 4 & 0 & 0 \\ -2 & 2 & 0 & 0 & 4 & 0 \\ 0 & 0 & 0 & 0 & 0 & 4 \end{pmatrix}, \qquad \#43\quad \begin{pmatrix} 4 & 2 & 2 & -2 & 0 & 0 \\ 2 & 4 & 0 & -2 & 1 & -1 \\ 2 & 0 & 4 & -2 & -1 & 1 \\ -2 & -2 & -2 & 4 & 1 & -1 \\ 0 & 1 & -1 & 1 & 4 & -2 \\ 0 & -1 & 1 & -1 & -2 & 4 \end{pmatrix},$$

$$\#44\quad \begin{pmatrix} 4 & -2 & 2 & -2 & 0 & 1 \\ -2 & 4 & 0 & 0 & -1 & -2 \\ 2 & 0 & 4 & 0 & 1 & -1 \\ -2 & 0 & 0 & 4 & 2 & 0 \\ 0 & -1 & 1 & 2 & 4 & -1 \\ 1 & -2 & -1 & 0 & -1 & 4 \end{pmatrix}, \qquad \#45\quad \begin{pmatrix} 4 & 1 & -2 & 2 & 2 & 1 \\ 1 & 4 & -2 & 1 & 1 & 0 \\ -2 & -2 & 4 & -2 & -2 & 0 \\ 2 & 1 & -2 & 4 & 0 & -1 \\ 2 & 1 & -2 & 0 & 4 & 1 \\ 1 & 0 & 0 & -1 & 1 & 4 \end{pmatrix},$$

$$\#46\ \begin{pmatrix} 4 & -1 & -2 & -2 & 2 & -1 \\ -1 & 4 & -1 & 2 & -2 & 2 \\ -2 & -1 & 4 & 1 & -1 & -1 \\ -2 & 2 & 1 & 4 & -1 & 0 \\ 2 & -2 & -1 & -1 & 4 & -2 \\ -1 & 2 & -1 & 0 & -2 & 4 \end{pmatrix}, \quad \#47\ \begin{pmatrix} 4 & -2 & -2 & 1 & -1 & 1 \\ -2 & 4 & 1 & -2 & 2 & -2 \\ -2 & 1 & 4 & -2 & -1 & 1 \\ 1 & -2 & -2 & 4 & -1 & 1 \\ -1 & 2 & -1 & -1 & 6 & 0 \\ 1 & -2 & 1 & 1 & 0 & 6 \end{pmatrix},$$

$$\#48\ \begin{pmatrix} 4 & -2 & 0 & 0 & 0 & 0 \\ -2 & 6 & -2 & -2 & -2 & 2 \\ 0 & -2 & 4 & 0 & 0 & 0 \\ 0 & -2 & 0 & 4 & 0 & 0 \\ 0 & -2 & 0 & 0 & 4 & 0 \\ 0 & 2 & 0 & 0 & 0 & 4 \end{pmatrix}, \quad \#49\ \begin{pmatrix} 4 & -2 & -2 & 2 & 0 & 0 \\ -2 & 4 & 2 & 0 & 0 & 0 \\ -2 & 2 & 4 & -2 & 0 & 0 \\ 2 & 0 & -2 & 4 & 0 & 0 \\ 0 & 0 & 0 & 0 & 4 & 0 \\ 0 & 0 & 0 & 0 & 0 & 4 \end{pmatrix}, \quad \#50\ \begin{pmatrix} 4 & 2 & 0 & 0 & 0 & 0 \\ 2 & 4 & 0 & 0 & 0 & 0 \\ 0 & 0 & 4 & -2 & 0 & 0 \\ 0 & 0 & -2 & 4 & 0 & 0 \\ 0 & 0 & 0 & 0 & 4 & -2 \\ 0 & 0 & 0 & 0 & -2 & 4 \end{pmatrix},$$

$$\#51\ \begin{pmatrix} 4 & 0 & 0 & 0 & 0 & 2 \\ 0 & 4 & 2 & -2 & 2 & 0 \\ 0 & 2 & 4 & 0 & 0 & 0 \\ 0 & -2 & 0 & 4 & 0 & 0 \\ 0 & 2 & 0 & 0 & 4 & 0 \\ 2 & 0 & 0 & 0 & 0 & 4 \end{pmatrix}, \quad \#52\ \begin{pmatrix} 4 & 2 & 2 & -1 & -1 & -2 \\ 2 & 4 & 0 & 1 & -2 & 0 \\ 2 & 0 & 4 & 0 & -1 & -1 \\ -1 & 1 & 0 & 4 & 0 & 2 \\ -1 & -2 & -1 & 0 & 4 & -1 \\ -2 & 0 & -1 & 2 & -1 & 4 \end{pmatrix}, \quad \#53\ \begin{pmatrix} 4 & 1 & -2 & 1 & -2 & -1 \\ 1 & 4 & -1 & 2 & 1 & 1 \\ -2 & -1 & 4 & -2 & 1 & -1 \\ 1 & 2 & -2 & 4 & 0 & 0 \\ -2 & 1 & 1 & 0 & 4 & 0 \\ -1 & 1 & -1 & 0 & 0 & 4 \end{pmatrix},$$

$$\#54\ \begin{pmatrix} 4 & -2 & -2 & 0 & 0 & 0 \\ -2 & 4 & 2 & 0 & 0 & 0 \\ -2 & 2 & 4 & 0 & 0 & 0 \\ 0 & 0 & 0 & 4 & 0 & 0 \\ 0 & 0 & 0 & 0 & 4 & 0 \\ 0 & 0 & 0 & 0 & 0 & 4 \end{pmatrix}, \quad \#55\ \begin{pmatrix} 4 & 1 & -1 & -1 & -2 & -2 \\ 1 & 4 & -1 & -2 & 1 & 0 \\ -1 & -1 & 4 & -1 & 1 & 2 \\ -1 & -2 & -1 & 4 & -1 & 0 \\ -2 & 1 & 1 & -1 & 4 & 2 \\ -2 & 0 & 2 & 0 & 2 & 4 \end{pmatrix}, \quad \#56\ \begin{pmatrix} 4 & -2 & 0 & 0 & 0 & 0 \\ -2 & 6 & -2 & -2 & 2 & 2 \\ 0 & -2 & 4 & 0 & 0 & 0 \\ 0 & -2 & 0 & 4 & 0 & 0 \\ 0 & 2 & 0 & 0 & 4 & 0 \\ 0 & 2 & 0 & 0 & 0 & 4 \end{pmatrix},$$

$$\#57\ \begin{pmatrix} 4 & 0 & 0 & 0 & 0 & 0 \\ 0 & 4 & 0 & 0 & 0 & 0 \\ 0 & 0 & 4 & 0 & 0 & 0 \\ 0 & 0 & 0 & 4 & 0 & 0 \\ 0 & 0 & 0 & 0 & 4 & 0 \\ 0 & 0 & 0 & 0 & 0 & 4 \end{pmatrix}, \quad \#58\ \begin{pmatrix} 4 & -2 & 0 & 0 & 0 & 0 \\ -2 & 6 & 2 & -2 & 2 & 0 \\ 0 & 2 & 4 & 0 & 0 & 0 \\ 0 & -2 & 0 & 4 & 0 & 0 \\ 0 & 2 & 0 & 0 & 4 & 0 \\ 0 & 0 & 0 & 0 & 0 & 4 \end{pmatrix}, \quad \#59\ \begin{pmatrix} 4 & -2 & -2 & -2 & -2 & -2 \\ -2 & 4 & 2 & 2 & 0 & 2 \\ -2 & 2 & 4 & 0 & 2 & 0 \\ -2 & 2 & 0 & 4 & 0 & 2 \\ -2 & 0 & 2 & 0 & 6 & 0 \\ -2 & 2 & 0 & 2 & 0 & 6 \end{pmatrix},$$

$$\#60\ \begin{pmatrix} 4 & 2 & -2 & 2 & -2 & -2 \\ 2 & 4 & 0 & 0 & -2 & -2 \\ -2 & 0 & 4 & -2 & 0 & 2 \\ 2 & 0 & -2 & 4 & 0 & 0 \\ -2 & -2 & 0 & 0 & 4 & 0 \\ -2 & -2 & 2 & 0 & 0 & 6 \end{pmatrix}, \quad \#61\ \begin{pmatrix} 4 & -2 & -2 & -2 & -2 & -2 \\ -2 & 6 & 2 & 0 & 2 & 2 \\ -2 & 2 & 6 & 2 & 0 & 0 \\ -2 & 0 & 2 & 6 & 2 & 2 \\ -2 & 2 & 0 & 2 & 6 & 0 \\ -2 & 2 & 0 & 2 & 0 & 6 \end{pmatrix},$$

$$\#62\ \begin{pmatrix} 8 & -4 & -4 & -2 & 2 & -2 \\ -4 & 8 & 2 & -2 & -4 & -2 \\ -4 & 2 & 8 & -2 & 2 & -2 \\ -2 & -2 & -2 & 8 & -2 & 2 \\ 2 & -4 & 2 & -2 & 8 & -2 \\ -2 & -2 & -2 & 2 & -2 & 8 \end{pmatrix}, \quad \#63\ \begin{pmatrix} 4 & -2 & -2 & -2 & -2 & -2 \\ -2 & 4 & 2 & 2 & 2 & 0 \\ -2 & 2 & 4 & 2 & 2 & 0 \\ -2 & 2 & 2 & 6 & 0 & 2 \\ -2 & 2 & 2 & 0 & 6 & 2 \\ -2 & 0 & 0 & 2 & 2 & 6 \end{pmatrix}, \quad \#64\ \begin{pmatrix} 4 & 0 & 0 & 0 & 0 & 0 \\ 0 & 4 & 0 & 0 & 0 & 0 \\ 0 & 0 & 4 & 0 & 0 & 0 \\ 0 & 0 & 0 & 4 & 0 & 0 \\ 0 & 0 & 0 & 0 & 4 & 0 \\ 0 & 0 & 0 & 0 & 0 & 4 \end{pmatrix},$$

$$\#65\ \begin{pmatrix} 4 & -2 & -2 & -2 & 2 \\ -2 & 4 & 2 & 0 & 0 \\ -2 & 2 & 4 & 0 & -2 \\ -2 & 0 & 0 & 4 & -2 \\ 2 & 0 & -2 & -2 & 4 \end{pmatrix}, \quad \#66\ \begin{pmatrix} 4 & -2 & -2 & -2 & -2 \\ -2 & 4 & 2 & 2 & 2 \\ -2 & 2 & 4 & 2 & 2 \\ -2 & 2 & 2 & 4 & 2 \\ -2 & 2 & 2 & 2 & 4 \end{pmatrix}, \quad \#67\ \begin{pmatrix} 4 & 2 & -2 & -2 & 0 \\ 2 & 4 & -2 & 0 & 0 \\ -2 & -2 & 4 & 2 & 0 \\ -2 & 0 & 2 & 4 & 0 \\ 0 & 0 & 0 & 0 & 4 \end{pmatrix},$$

$$\#68\ \begin{pmatrix} 4 & -1 & -2 & -2 & 2 \\ -1 & 4 & -1 & 2 & 1 \\ -2 & -1 & 4 & 1 & -1 \\ -2 & 2 & 1 & 4 & -1 \\ 2 & 1 & -1 & -1 & 4 \end{pmatrix}, \quad \#69\ \begin{pmatrix} 4 & 2 & 1 & -2 & -2 \\ 2 & 4 & -1 & -2 & 0 \\ 1 & -1 & 4 & -1 & -2 \\ -2 & -2 & -1 & 4 & 2 \\ -2 & 0 & -2 & 2 & 4 \end{pmatrix}, \quad \#70\ \begin{pmatrix} 4 & 0 & -1 & -1 & 2 \\ 0 & 4 & -2 & -2 & 0 \\ -1 & -2 & 4 & 0 & 0 \\ -1 & -2 & 0 & 4 & 0 \\ 2 & 0 & 0 & 0 & 4 \end{pmatrix},$$

$$\#71\ \begin{pmatrix} 4 & -2 & -2 & -2 & 0 \\ -2 & 4 & 0 & 2 & 0 \\ -2 & 0 & 4 & 2 & 0 \\ -2 & 2 & 2 & 4 & 0 \\ 0 & 0 & 0 & 0 & 4 \end{pmatrix}, \quad \#72\ \begin{pmatrix} 4 & -2 & -2 & 1 & 1 \\ -2 & 4 & 2 & -1 & 1 \\ -2 & 2 & 4 & -2 & -1 \\ 1 & -1 & -2 & 4 & 2 \\ 1 & 1 & -1 & 2 & 4 \end{pmatrix}, \quad \#73\ \begin{pmatrix} 4 & 1 & 2 & 1 & 0 \\ 1 & 4 & 2 & 2 & -1 \\ 2 & 2 & 4 & 2 & 0 \\ 1 & 2 & 2 & 4 & 1 \\ 0 & -1 & 0 & 1 & 4 \end{pmatrix},$$

$$\#74\ \begin{pmatrix} 4 & -1 & 1 & 1 & 0 \\ -1 & 4 & -2 & -2 & 1 \\ 1 & -2 & 4 & 0 & -1 \\ 1 & -2 & 0 & 4 & -1 \\ 0 & 1 & -1 & -1 & 4 \end{pmatrix}, \quad \#75\ \begin{pmatrix} 4 & -2 & -2 & 2 & 2 \\ -2 & 4 & 2 & -2 & -2 \\ -2 & 2 & 4 & 0 & -2 \\ 2 & -2 & 0 & 4 & 0 \\ 2 & -2 & -2 & 0 & 8 \end{pmatrix}, \quad \#76\ \begin{pmatrix} 4 & -2 & -2 & -2 & 1 \\ -2 & 4 & 2 & 0 & 0 \\ -2 & 2 & 4 & 2 & 1 \\ -2 & 0 & 2 & 4 & 0 \\ 1 & 0 & 1 & 0 & 4 \end{pmatrix},$$

$$\#77\ \begin{pmatrix} 4 & -2 & -2 & 2 & -2 \\ -2 & 4 & 0 & 0 & 1 \\ -2 & 0 & 4 & -1 & 0 \\ 2 & 0 & -1 & 4 & -2 \\ -2 & 1 & 0 & -2 & 4 \end{pmatrix}, \quad \#78\ \begin{pmatrix} 4 & 0 & 0 & 0 & 0 \\ 0 & 4 & 0 & 0 & 0 \\ 0 & 0 & 4 & 0 & 0 \\ 0 & 0 & 0 & 4 & 0 \\ 0 & 0 & 0 & 0 & 4 \end{pmatrix}, \quad \#79\ \begin{pmatrix} 4 & 2 & -2 & -2 & 0 \\ 2 & 4 & -2 & -2 & 0 \\ -2 & -2 & 4 & 0 & 0 \\ -2 & -2 & 0 & 4 & 0 \\ 0 & 0 & 0 & 0 & 8 \end{pmatrix},$$

$$\#80\ \begin{pmatrix} 4 & -2 & 0 & 0 & 0 \\ -2 & 6 & 2 & 2 & 2 \\ 0 & 2 & 4 & 0 & 0 \\ 0 & 2 & 0 & 4 & 0 \\ 0 & 2 & 0 & 0 & 4 \end{pmatrix}, \quad \#81\ \begin{pmatrix} 4 & -2 & -2 & 0 & 0 \\ -2 & 4 & 0 & 0 & 0 \\ -2 & 0 & 4 & 0 & 0 \\ 0 & 0 & 0 & 4 & 0 \\ 0 & 0 & 0 & 0 & 4 \end{pmatrix}, \quad \#82\ \begin{pmatrix} 4 & -2 & 1 & -1 & 0 \\ -2 & 4 & 0 & -1 & -1 \\ 1 & 0 & 4 & -2 & 1 \\ -1 & -1 & -2 & 4 & -1 \\ 0 & -1 & 1 & -1 & 4 \end{pmatrix},$$

$$\#83\ \begin{pmatrix} 4 & 2 & 0 & 0 & 0 \\ 2 & 4 & 0 & 0 & 0 \\ 0 & 0 & 4 & 2 & 0 \\ 0 & 0 & 2 & 4 & 0 \\ 0 & 0 & 0 & 0 & 4 \end{pmatrix}, \quad \#84\ \begin{pmatrix} 4 & -2 & -2 & -2 & 2 \\ -2 & 4 & 2 & 1 & -1 \\ -2 & 2 & 4 & 2 & -2 \\ -2 & 1 & 2 & 4 & -1 \\ 2 & -1 & -2 & -1 & 4 \end{pmatrix}, \quad \#85\ \begin{pmatrix} 4 & -2 & -1 & 2 & 2 \\ -2 & 4 & -1 & -1 & -1 \\ -1 & -1 & 4 & -2 & -2 \\ 2 & -1 & -2 & 4 & 1 \\ 2 & -1 & -2 & 1 & 6 \end{pmatrix},$$

$$\#86 \begin{pmatrix} 4 & 0 & 0 & 0 & 0 \\ 0 & 4 & 0 & 0 & 0 \\ 0 & 0 & 4 & 0 & 0 \\ 0 & 0 & 0 & 4 & 0 \\ 0 & 0 & 0 & 0 & 4 \end{pmatrix}, \quad \#87 \begin{pmatrix} 4 & -1 & -1 & 0 & 1 \\ -1 & 4 & -1 & 1 & 0 \\ -1 & -1 & 4 & 1 & 1 \\ 0 & 1 & 1 & 4 & -1 \\ 1 & 0 & 1 & -1 & 4 \end{pmatrix}, \quad \#88 \begin{pmatrix} 4 & 2 & 0 & 0 & 0 \\ 2 & 4 & 0 & 0 & 0 \\ 0 & 0 & 4 & 0 & 0 \\ 0 & 0 & 0 & 4 & 0 \\ 0 & 0 & 0 & 0 & 4 \end{pmatrix}, \quad \#89 \begin{pmatrix} 4 & 2 & 2 & 2 & 2 \\ 2 & 4 & 2 & 2 & 2 \\ 2 & 2 & 4 & 0 & 0 \\ 2 & 2 & 0 & 6 & 2 \\ 2 & 2 & 0 & 2 & 6 \end{pmatrix},$$

$$\#90 \begin{pmatrix} 4 & -2 & 2 & -2 & -2 \\ -2 & 4 & -2 & 2 & 2 \\ 2 & -2 & 4 & 0 & 0 \\ -2 & 2 & 0 & 8 & 2 \\ -2 & 2 & 0 & 2 & 8 \end{pmatrix}, \quad \#91 \begin{pmatrix} 4 & 0 & 0 & 0 & 0 \\ 0 & 4 & 0 & 0 & 0 \\ 0 & 0 & 4 & 0 & 0 \\ 0 & 0 & 0 & 4 & 0 \\ 0 & 0 & 0 & 0 & 4 \end{pmatrix}, \quad \#92 \begin{pmatrix} 4 & 2 & 0 & 0 & 0 \\ 2 & 6 & 0 & 2 & -2 \\ 0 & 0 & 4 & -2 & -2 \\ 0 & 2 & -2 & 4 & 0 \\ 0 & -2 & -2 & 0 & 4 \end{pmatrix},$$

$$\#93 \begin{pmatrix} 4 & 0 & 0 & 0 & 0 \\ 0 & 4 & 0 & 0 & 0 \\ 0 & 0 & 4 & 0 & 0 \\ 0 & 0 & 0 & 4 & 0 \\ 0 & 0 & 0 & 0 & 8 \end{pmatrix}, \quad \#94 \begin{pmatrix} 4 & -2 & 2 & 2 & 2 \\ -2 & 4 & -2 & -2 & -2 \\ 2 & -2 & 4 & 0 & 2 \\ 2 & -2 & 0 & 4 & 2 \\ 2 & -2 & 2 & 2 & 6 \end{pmatrix}, \quad \#95 \begin{pmatrix} 4 & -2 & 0 & 0 & -2 \\ -2 & 6 & 0 & -2 & 2 \\ 0 & 0 & 4 & 0 & 0 \\ 0 & -2 & 0 & 4 & -2 \\ -2 & 2 & 0 & -2 & 6 \end{pmatrix},$$

$$\#96 \begin{pmatrix} 8 & 2 & -4 & 4 & -4 \\ 2 & 8 & 2 & 4 & -4 \\ -4 & 2 & 8 & -2 & 2 \\ 4 & 4 & -2 & 8 & -2 \\ -4 & -4 & 2 & -2 & 8 \end{pmatrix}, \quad \#97 \begin{pmatrix} 4 & -2 & -2 & -2 & -2 \\ -2 & 4 & 2 & 0 & 2 \\ -2 & 2 & 4 & 0 & 2 \\ -2 & 0 & 0 & 6 & 2 \\ -2 & 2 & 2 & 2 & 6 \end{pmatrix}, \quad \#98 \begin{pmatrix} 4 & 2 & -2 & -2 & 2 \\ 2 & 6 & -2 & -2 & 0 \\ -2 & -2 & 6 & 0 & -2 \\ -2 & -2 & 0 & 6 & -2 \\ 2 & 0 & -2 & -2 & 6 \end{pmatrix},$$

$$\#99 \begin{pmatrix} 4 & -2 & -2 & -2 \\ -2 & 4 & 2 & 2 \\ -2 & 2 & 4 & 0 \\ -2 & 2 & 0 & 4 \end{pmatrix}, \quad \#100 \begin{pmatrix} 4 & -2 & -2 & 2 \\ -2 & 4 & 0 & 0 \\ -2 & 0 & 4 & -2 \\ 2 & 0 & -2 & 4 \end{pmatrix}, \quad \#101 \begin{pmatrix} 4 & -1 & -2 & -2 \\ -1 & 4 & 2 & 2 \\ -2 & 2 & 4 & 1 \\ -2 & 2 & 1 & 4 \end{pmatrix},$$

$$\#102 \begin{pmatrix} 4 & -2 & 2 & -2 \\ -2 & 4 & 0 & 1 \\ 2 & 0 & 4 & -2 \\ -2 & 1 & -2 & 4 \end{pmatrix}, \quad \#103 \begin{pmatrix} 4 & -2 & -2 & 0 \\ -2 & 4 & 2 & 0 \\ -2 & 2 & 4 & 0 \\ 0 & 0 & 0 & 4 \end{pmatrix}, \quad \#104 \begin{pmatrix} 4 & 2 & 0 & 0 \\ 2 & 4 & 0 & 0 \\ 0 & 0 & 4 & -2 \\ 0 & 0 & -2 & 4 \end{pmatrix},$$

$$\#105 \begin{pmatrix} 4 & -2 & -2 & 2 \\ -2 & 4 & 0 & -2 \\ -2 & 0 & 4 & -2 \\ 2 & -2 & -2 & 8 \end{pmatrix}, \quad \#106 \begin{pmatrix} 4 & -2 & -2 & 1 \\ -2 & 4 & 0 & 1 \\ -2 & 0 & 4 & -1 \\ 1 & 1 & -1 & 4 \end{pmatrix}, \quad \#107 \begin{pmatrix} 4 & 0 & 0 & 0 \\ 0 & 4 & 0 & 0 \\ 0 & 0 & 4 & 0 \\ 0 & 0 & 0 & 4 \end{pmatrix},$$

$$\#108 \begin{pmatrix} 4 & 1 & -2 & 1 \\ 1 & 4 & 1 & -1 \\ -2 & 1 & 4 & -2 \\ 1 & -1 & -2 & 4 \end{pmatrix}, \quad \#109 \begin{pmatrix} 4 & 1 & -2 & 1 \\ 1 & 4 & -2 & 1 \\ -2 & -2 & 4 & -2 \\ 1 & 1 & -2 & 4 \end{pmatrix}, \quad \#110 \begin{pmatrix} 4 & 0 & 0 & 1 \\ 0 & 4 & 0 & 1 \\ 0 & 0 & 4 & -2 \\ 1 & 1 & -2 & 4 \end{pmatrix},$$

$$\#111 \begin{pmatrix} 4 & -2 & -2 & 0 \\ -2 & 4 & 2 & 1 \\ -2 & 2 & 4 & 1 \\ 0 & 1 & 1 & 4 \end{pmatrix}, \quad \#112 \begin{pmatrix} 4 & 0 & -1 & 1 \\ 0 & 4 & 1 & -1 \\ -1 & 1 & 4 & 0 \\ 1 & -1 & 0 & 4 \end{pmatrix}, \quad \#113 \begin{pmatrix} 4 & -2 & -2 & -2 \\ -2 & 4 & 0 & 2 \\ -2 & 0 & 4 & 2 \\ -2 & 2 & 2 & 8 \end{pmatrix},$$

$$\#114 \begin{pmatrix} 6 & -3 & -3 & 3 \\ -3 & 6 & 3 & 0 \\ -3 & 3 & 6 & -3 \\ 3 & 0 & -3 & 6 \end{pmatrix}, \quad \#115 \begin{pmatrix} 4 & -2 & 2 & 0 \\ -2 & 4 & -2 & 0 \\ 2 & -2 & 4 & 0 \\ 0 & 0 & 0 & 8 \end{pmatrix}, \quad \#116 \begin{pmatrix} 4 & 0 & -2 & -2 \\ 0 & 4 & 2 & 2 \\ -2 & 2 & 6 & 2 \\ -2 & 2 & 2 & 6 \end{pmatrix},$$

$$\#117 \begin{pmatrix} 4 & 0 & 0 & 0 \\ 0 & 4 & 0 & 0 \\ 0 & 0 & 4 & 0 \\ 0 & 0 & 0 & 4 \end{pmatrix}, \quad \#118 \begin{pmatrix} 4 & -1 & 2 & -1 \\ -1 & 4 & -2 & 1 \\ 2 & -2 & 4 & -2 \\ -1 & 1 & -2 & 6 \end{pmatrix}, \quad \#119 \begin{pmatrix} 4 & -2 & 1 & -1 \\ -2 & 4 & -2 & 0 \\ 1 & -2 & 4 & 1 \\ -1 & 0 & 1 & 4 \end{pmatrix}, \quad \#120 \begin{pmatrix} 4 & 2 & 0 & 1 \\ 2 & 4 & 1 & 1 \\ 0 & 1 & 4 & 2 \\ 1 & 1 & 2 & 4 \end{pmatrix},$$

$$\#121 \begin{pmatrix} 4 & -2 & -1 & -1 \\ -2 & 4 & -1 & -1 \\ -1 & -1 & 6 & 0 \\ -1 & -1 & 0 & 6 \end{pmatrix}, \quad \#122 \begin{pmatrix} 4 & 1 & 1 & 1 \\ 1 & 4 & -1 & -1 \\ 1 & -1 & 4 & -1 \\ 1 & -1 & -1 & 4 \end{pmatrix}, \quad \#123 \begin{pmatrix} 4 & 0 & 0 & -2 \\ 0 & 4 & 0 & -2 \\ 0 & 0 & 4 & -2 \\ -2 & -2 & -2 & 6 \end{pmatrix},$$

$$\#124 \begin{pmatrix} 4 & -2 & -2 & 2 \\ -2 & 4 & 0 & -2 \\ -2 & 0 & 4 & -2 \\ 2 & -2 & -2 & 6 \end{pmatrix}, \quad \#125 \begin{pmatrix} 4 & 0 & 0 & 0 \\ 0 & 4 & 0 & 2 \\ 0 & 0 & 4 & -2 \\ 0 & 2 & -2 & 8 \end{pmatrix}, \quad \#126 \begin{pmatrix} 4 & -2 & 0 & 0 \\ -2 & 4 & 0 & 0 \\ 0 & 0 & 4 & 0 \\ 0 & 0 & 0 & 4 \end{pmatrix}, \quad \#127 \begin{pmatrix} 4 & -2 & 0 & 0 \\ -2 & 4 & 0 & 0 \\ 0 & 0 & 4 & 2 \\ 0 & 0 & 2 & 4 \end{pmatrix},$$

$$\#128 \begin{pmatrix} 4 & 2 & 2 & -1 \\ 2 & 4 & 1 & -2 \\ 2 & 1 & 6 & 2 \\ -1 & -2 & 2 & 6 \end{pmatrix}, \quad \#129 \begin{pmatrix} 4 & 1 & 1 & 0 \\ 1 & 4 & 0 & 1 \\ 1 & 0 & 4 & -1 \\ 0 & 1 & -1 & 4 \end{pmatrix}, \quad \#130 \begin{pmatrix} 4 & 0 & 0 & 0 \\ 0 & 4 & 0 & 0 \\ 0 & 0 & 4 & 0 \\ 0 & 0 & 0 & 8 \end{pmatrix}, \quad \#131 \begin{pmatrix} 4 & -2 & 0 & -2 \\ -2 & 6 & -2 & 0 \\ 0 & -2 & 4 & 2 \\ -2 & 0 & 2 & 6 \end{pmatrix},$$

$$\#132 \begin{pmatrix} 4 & 0 & 0 & 0 \\ 0 & 4 & 0 & 0 \\ 0 & 0 & 4 & 0 \\ 0 & 0 & 0 & 4 \end{pmatrix}, \quad \#133 \begin{pmatrix} 4 & 2 & -2 & 2 \\ 2 & 4 & -2 & 0 \\ -2 & -2 & 4 & 0 \\ 2 & 0 & 0 & 6 \end{pmatrix}, \quad \#134 \begin{pmatrix} 4 & 1 & -2 & -1 \\ 1 & 4 & -2 & -1 \\ -2 & -2 & 6 & 2 \\ -1 & -1 & 2 & 4 \end{pmatrix},$$

$$\#135 \begin{pmatrix} 4 & -2 & 0 & 0 \\ -2 & 4 & 0 & 0 \\ 0 & 0 & 8 & -4 \\ 0 & 0 & -4 & 8 \end{pmatrix}, \quad \#136 \begin{pmatrix} 4 & -2 & 2 & -2 \\ -2 & 4 & -2 & 2 \\ 2 & -2 & 8 & 2 \\ -2 & 2 & 2 & 8 \end{pmatrix}, \quad \#137 \begin{pmatrix} 4 & -2 & -2 & -2 \\ -2 & 4 & 2 & 2 \\ -2 & 2 & 6 & 0 \\ -2 & 2 & 0 & 6 \end{pmatrix},$$

$$\#138 \begin{pmatrix} 6 & -3 & 0 & 0 \\ -3 & 6 & 0 & 0 \\ 0 & 0 & 6 & 3 \\ 0 & 0 & 3 & 6 \end{pmatrix}, \quad \#139 \begin{pmatrix} 4 & 0 & -2 & -2 \\ 0 & 4 & -2 & -2 \\ -2 & -2 & 8 & 2 \\ -2 & -2 & 2 & 8 \end{pmatrix}, \quad \#140 \begin{pmatrix} 8 & 2 & -4 & -4 \\ 2 & 8 & -4 & 2 \\ -4 & -4 & 8 & 2 \\ -4 & 2 & 2 & 8 \end{pmatrix},$$

#141 $\begin{pmatrix} 4 & 2 & -2 & -2 \\ 2 & 6 & -2 & 0 \\ -2 & -2 & 6 & 2 \\ -2 & 0 & 2 & 6 \end{pmatrix}$, #142 $\begin{pmatrix} 8 & 2 & -4 & -4 \\ 2 & 8 & -4 & 2 \\ -4 & -4 & 8 & 2 \\ -4 & 2 & 2 & 8 \end{pmatrix}$, #143 $\begin{pmatrix} 4 & 0 & 0 & 0 \\ 0 & 6 & 2 & -2 \\ 0 & 2 & 6 & 2 \\ 0 & -2 & 2 & 6 \end{pmatrix}$,

#144 $\begin{pmatrix} 6 & -3 & -3 & 3 \\ -3 & 6 & 3 & 0 \\ -3 & 3 & 6 & -3 \\ 3 & 0 & -3 & 6 \end{pmatrix}$, #145 $\begin{pmatrix} 8 & 2 & -4 & 0 \\ 2 & 8 & -4 & 0 \\ -4 & -4 & 8 & 0 \\ 0 & 0 & 0 & 4 \end{pmatrix}$, #146 $\begin{pmatrix} 4 & -2 & -2 & 0 \\ -2 & 4 & 0 & 0 \\ -2 & 0 & 4 & 0 \\ 0 & 0 & 0 & 12 \end{pmatrix}$,

#147 $\begin{pmatrix} 8 & -4 & -4 & -4 \\ -4 & 8 & 4 & 4 \\ -4 & 4 & 8 & 0 \\ -4 & 4 & 0 & 8 \end{pmatrix}$, #148 $\begin{pmatrix} 4 & -2 & 0 & -2 \\ -2 & 6 & 0 & 2 \\ 0 & 0 & 4 & 0 \\ -2 & 2 & 0 & 6 \end{pmatrix}$, #149 $\begin{pmatrix} 4 & 0 & 0 & 2 \\ 0 & 4 & 2 & 0 \\ 0 & 2 & 6 & 0 \\ 2 & 0 & 0 & 6 \end{pmatrix}$, #150 $\begin{pmatrix} 6 & 0 & 0 & 0 \\ 0 & 6 & 0 & 0 \\ 0 & 0 & 6 & 0 \\ 0 & 0 & 0 & 6 \end{pmatrix}$,

#151 $\begin{pmatrix} 4 & -2 & 0 & 0 \\ -2 & 4 & 0 & 0 \\ 0 & 0 & 6 & 0 \\ 0 & 0 & 0 & 6 \end{pmatrix}$, #152 $\begin{pmatrix} 4 & -2 & 0 & 0 \\ -2 & 6 & 0 & -2 \\ 0 & 0 & 4 & 0 \\ 0 & -2 & 0 & 4 \end{pmatrix}$, #153 $\begin{pmatrix} 4 & 0 & 0 & 0 \\ 0 & 4 & 0 & 0 \\ 0 & 0 & 8 & 0 \\ 0 & 0 & 0 & 8 \end{pmatrix}$, #154 $\begin{pmatrix} 4 & -2 & -2 & 0 \\ -2 & 6 & 0 & 2 \\ -2 & 0 & 6 & 2 \\ 0 & 2 & 2 & 8 \end{pmatrix}$,

#155 $\begin{pmatrix} 12 & -6 & -6 & 6 \\ -6 & 12 & 6 & -6 \\ -6 & 6 & 12 & 0 \\ 6 & -6 & 0 & 12 \end{pmatrix}$, #156 $\begin{pmatrix} 12 & -6 & 6 & -6 \\ -6 & 12 & -6 & 6 \\ 6 & -6 & 12 & 0 \\ -6 & 6 & 0 & 12 \end{pmatrix}$, #157 $\begin{pmatrix} 4 & -2 & 2 & -2 \\ -2 & 10 & -4 & -2 \\ 2 & -4 & 10 & -4 \\ -2 & -2 & -4 & 10 \end{pmatrix}$,

#158 $\begin{pmatrix} 8 & 2 & 4 & 2 \\ 2 & 8 & -2 & 2 \\ 4 & -2 & 8 & -2 \\ 2 & 2 & -2 & 8 \end{pmatrix}$, #159 $\begin{pmatrix} 8 & -2 & 2 & 2 \\ -2 & 8 & 2 & 2 \\ 2 & 2 & 8 & -2 \\ 2 & 2 & -2 & 8 \end{pmatrix}$, #160 $\begin{pmatrix} 4 & 0 & 0 & 0 \\ 0 & 4 & 0 & 0 \\ 0 & 0 & 8 & 0 \\ 0 & 0 & 0 & 8 \end{pmatrix}$, #161 $\begin{pmatrix} 6 & 0 & 0 & 0 \\ 0 & 6 & 0 & 0 \\ 0 & 0 & 6 & 0 \\ 0 & 0 & 0 & 6 \end{pmatrix}$,

#162 $\begin{pmatrix} 4 & -2 & -2 \\ -2 & 4 & 2 \\ -2 & 2 & 4 \end{pmatrix}$, #163 $\begin{pmatrix} 4 & -1 & -2 \\ -1 & 4 & 2 \\ -2 & 2 & 4 \end{pmatrix}$, #164 $\begin{pmatrix} 4 & 0 & 0 \\ 0 & 4 & 0 \\ 0 & 0 & 4 \end{pmatrix}$, #165 $\begin{pmatrix} 4 & -2 & 1 \\ -2 & 4 & 0 \\ 1 & 0 & 4 \end{pmatrix}$,

#166 $\begin{pmatrix} 4 & -2 & 0 \\ -2 & 4 & 0 \\ 0 & 0 & 4 \end{pmatrix}$, #167 $\begin{pmatrix} 4 & 1 & -1 \\ 1 & 4 & 1 \\ -1 & 1 & 4 \end{pmatrix}$, #168 $\begin{pmatrix} 4 & -2 & -2 \\ -2 & 4 & 2 \\ -2 & 2 & 8 \end{pmatrix}$, #169 $\begin{pmatrix} 4 & 1 & -1 \\ 1 & 4 & -1 \\ -1 & -1 & 4 \end{pmatrix}$,

#170 $\begin{pmatrix} 4 & 1 & 1 \\ 1 & 4 & 1 \\ 1 & 1 & 6 \end{pmatrix}$, #171 $\begin{pmatrix} 4 & -2 & -2 \\ -2 & 4 & 2 \\ -2 & 2 & 6 \end{pmatrix}$, #172 $\begin{pmatrix} 4 & 1 & 0 \\ 1 & 4 & 1 \\ 0 & 1 & 4 \end{pmatrix}$, #173 $\begin{pmatrix} 4 & 0 & 2 \\ 0 & 4 & 2 \\ 2 & 2 & 8 \end{pmatrix}$, #174 $\begin{pmatrix} 4 & 0 & 0 \\ 0 & 4 & 0 \\ 0 & 0 & 8 \end{pmatrix}$,

#175 $\begin{pmatrix} 4 & -2 & 1 \\ -2 & 4 & -2 \\ 1 & -2 & 6 \end{pmatrix}$, #176 $\begin{pmatrix} 4 & -2 & 0 \\ -2 & 4 & 0 \\ 0 & 0 & 12 \end{pmatrix}$, #177 $\begin{pmatrix} 4 & 0 & 0 \\ 0 & 8 & -4 \\ 0 & -4 & 8 \end{pmatrix}$, #178 $\begin{pmatrix} 4 & -2 & -2 \\ -2 & 6 & 2 \\ -2 & 2 & 6 \end{pmatrix}$,

#179 $\begin{pmatrix} 4 & -2 & 0 \\ -2 & 4 & 0 \\ 0 & 0 & 8 \end{pmatrix}$, #180 $\begin{pmatrix} 4 & -2 & 0 \\ -2 & 6 & 2 \\ 0 & 2 & 4 \end{pmatrix}$, #181 $\begin{pmatrix} 4 & 0 & 0 \\ 0 & 4 & 0 \\ 0 & 0 & 4 \end{pmatrix}$, #182 $\begin{pmatrix} 4 & 1 & -2 \\ 1 & 4 & 1 \\ -2 & 1 & 6 \end{pmatrix}$,

#183 $\begin{pmatrix} 4 & -1 & -1 \\ -1 & 6 & 2 \\ -1 & 2 & 6 \end{pmatrix}$, #184 $\begin{pmatrix} 6 & 2 & 2 \\ 2 & 6 & -2 \\ 2 & -2 & 6 \end{pmatrix}$, #185 $\begin{pmatrix} 4 & 0 & 0 \\ 0 & 4 & 0 \\ 0 & 0 & 8 \end{pmatrix}$, #186 $\begin{pmatrix} 6 & -3 & -3 \\ -3 & 6 & 3 \\ -3 & 3 & 6 \end{pmatrix}$,

#187 $\begin{pmatrix} 4 & -2 & 0 \\ -2 & 4 & 0 \\ 0 & 0 & 6 \end{pmatrix}$, #188 $\begin{pmatrix} 4 & 0 & 2 \\ 0 & 4 & 2 \\ 2 & 2 & 12 \end{pmatrix}$, #189 $\begin{pmatrix} 4 & 0 & 0 \\ 0 & 4 & 2 \\ 0 & 2 & 8 \end{pmatrix}$, #190 $\begin{pmatrix} 4 & 0 & 0 \\ 0 & 8 & -4 \\ 0 & -4 & 8 \end{pmatrix}$, #191 $\begin{pmatrix} 6 & 0 & 0 \\ 0 & 6 & 0 \\ 0 & 0 & 6 \end{pmatrix}$,

#192 $\begin{pmatrix} 4 & 0 & 0 \\ 0 & 8 & 0 \\ 0 & 0 & 8 \end{pmatrix}$, #193 $\begin{pmatrix} 4 & 2 & 0 \\ 2 & 6 & 0 \\ 0 & 0 & 4 \end{pmatrix}$, #194 $\begin{pmatrix} 4 & 0 & -2 \\ 0 & 6 & 0 \\ -2 & 0 & 6 \end{pmatrix}$, #195 $\begin{pmatrix} 8 & -4 & 2 \\ -4 & 8 & -4 \\ 2 & -4 & 8 \end{pmatrix}$,

#196 $\begin{pmatrix} 4 & 0 & 0 \\ 0 & 4 & 0 \\ 0 & 0 & 12 \end{pmatrix}$, #197 $\begin{pmatrix} 4 & 0 & 0 \\ 0 & 6 & -2 \\ 0 & -2 & 6 \end{pmatrix}$, #198 $\begin{pmatrix} 4 & -2 & 0 \\ -2 & 4 & 0 \\ 0 & 0 & 12 \end{pmatrix}$, #199 $\begin{pmatrix} 4 & 0 & 0 \\ 0 & 8 & 2 \\ 0 & 2 & 8 \end{pmatrix}$, #200 $\begin{pmatrix} 4 & 0 & 0 \\ 0 & 6 & 0 \\ 0 & 0 & 6 \end{pmatrix}$,

#201 $\begin{pmatrix} 6 & 0 & 0 \\ 0 & 6 & -3 \\ 0 & -3 & 6 \end{pmatrix}$, #202 $\begin{pmatrix} 4 & 0 & 0 \\ 0 & 8 & 0 \\ 0 & 0 & 8 \end{pmatrix}$, #203 $\begin{pmatrix} 4 & -2 & 0 \\ -2 & 6 & -2 \\ 0 & -2 & 8 \end{pmatrix}$, #204 $\begin{pmatrix} 8 & 2 & 2 \\ 2 & 8 & -2 \\ 2 & -2 & 8 \end{pmatrix}$,

#205 $\begin{pmatrix} 6 & 0 & 2 \\ 0 & 6 & 2 \\ 2 & 2 & 8 \end{pmatrix}$, #206 $\begin{pmatrix} 4 & 0 & 0 \\ 0 & 12 & 0 \\ 0 & 0 & 12 \end{pmatrix}$, #207 $\begin{pmatrix} 6 & 2 & -2 \\ 2 & 6 & 2 \\ -2 & 2 & 6 \end{pmatrix}$, #208 $\begin{pmatrix} 4 & -2 & -2 \\ -2 & 10 & 4 \\ -2 & 4 & 10 \end{pmatrix}$,

#209 $\begin{pmatrix} 8 & -2 & -2 \\ -2 & 8 & 2 \\ -2 & 2 & 8 \end{pmatrix}$, #210 $\begin{pmatrix} 12 & -6 & -6 \\ -6 & 12 & 6 \\ -6 & 6 & 12 \end{pmatrix}$, #211 $\begin{pmatrix} 6 & 0 & 0 \\ 0 & 6 & 0 \\ 0 & 0 & 6 \end{pmatrix}$, #212 $\begin{pmatrix} 6 & -2 & -2 \\ -2 & 6 & -2 \\ -2 & -2 & 8 \end{pmatrix}$,

#213 $\begin{pmatrix} 4 & 0 & 0 \\ 0 & 8 & 0 \\ 0 & 0 & 12 \end{pmatrix}$, #214 $\begin{pmatrix} 6 & 0 & 0 \\ 0 & 6 & 0 \\ 0 & 0 & 12 \end{pmatrix}$, #215 $\begin{pmatrix} 4 & 0 & 0 \\ 0 & 4 & 0 \\ 0 & 0 & 16 \end{pmatrix}$, #216 $\begin{pmatrix} 8 & 0 & 0 \\ 0 & 8 & 0 \\ 0 & 0 & 8 \end{pmatrix}$, #217 $\begin{pmatrix} 12 & -6 & -6 \\ -6 & 12 & 6 \\ -6 & 6 & 12 \end{pmatrix}$,

#218 $\begin{pmatrix} 8 & -4 & 0 \\ -4 & 8 & 0 \\ 0 & 0 & 12 \end{pmatrix}$, #219 $\begin{pmatrix} 12 & 0 & 0 \\ 0 & 12 & 0 \\ 0 & 0 & 12 \end{pmatrix}$, #220 $\begin{pmatrix} 6 & 2 & 2 \\ 2 & 10 & -4 \\ 2 & -4 & 10 \end{pmatrix}$, #221 $\begin{pmatrix} 8 & 0 & 0 \\ 0 & 8 & 0 \\ 0 & 0 & 8 \end{pmatrix}$,

#222 $\begin{pmatrix} 4 & -2 \\ -2 & 4 \end{pmatrix}$, #223 $\begin{pmatrix} 4 & 1 \\ 1 & 4 \end{pmatrix}$, #224 $\begin{pmatrix} 4 & 0 \\ 0 & 4 \end{pmatrix}$, #225 $\begin{pmatrix} 4 & 2 \\ 2 & 6 \end{pmatrix}$, #226 $\begin{pmatrix} 4 & 0 \\ 0 & 8 \end{pmatrix}$, #227 $\begin{pmatrix} 4 & 1 \\ 1 & 6 \end{pmatrix}$,

$\#228\ \begin{pmatrix} 6 & 0 \\ 0 & 6 \end{pmatrix}$, $\#229\ \begin{pmatrix} 4 & 0 \\ 0 & 6 \end{pmatrix}$, $\#230\ \begin{pmatrix} 6 & -3 \\ -3 & 6 \end{pmatrix}$, $\#231\ \begin{pmatrix} 8 & -4 \\ -4 & 8 \end{pmatrix}$, $\#232\ \begin{pmatrix} 4 & -2 \\ -2 & 8 \end{pmatrix}$, $\#233\ \begin{pmatrix} 4 & -2 \\ -2 & 12 \end{pmatrix}$, $\#234\ \begin{pmatrix} 4 & 0 \\ 0 & 12 \end{pmatrix}$, $\#235\ \begin{pmatrix} 6 & -2 \\ -2 & 6 \end{pmatrix}$, $\#236\ \begin{pmatrix} 4 & 0 \\ 0 & 8 \end{pmatrix}$, $\#237\ \begin{pmatrix} 4 & -2 \\ -2 & 16 \end{pmatrix}$, $\#238\ \begin{pmatrix} 8 & 0 \\ 0 & 8 \end{pmatrix}$, $\#239\ \begin{pmatrix} 8 & 4 \\ 4 & 12 \end{pmatrix}$, $\#240\ \begin{pmatrix} 6 & -3 \\ -3 & 12 \end{pmatrix}$, $\#241\ \begin{pmatrix} 4 & 2 \\ 2 & 10 \end{pmatrix}$, $\#242\ \begin{pmatrix} 6 & 0 \\ 0 & 6 \end{pmatrix}$, $\#243\ \begin{pmatrix} 6 & 2 \\ 2 & 10 \end{pmatrix}$, $\#244\ \begin{pmatrix} 4 & 0 \\ 0 & 24 \end{pmatrix}$, $\#245\ \begin{pmatrix} 12 & -6 \\ -6 & 12 \end{pmatrix}$, $\#246\ \begin{pmatrix} 8 & -2 \\ -2 & 8 \end{pmatrix}$, $\#247\ \begin{pmatrix} 12 & 0 \\ 0 & 12 \end{pmatrix}$, $\#248\ \begin{pmatrix} 8 & 0 \\ 0 & 12 \end{pmatrix}$, $\#249\ \begin{pmatrix} 8 & -4 \\ -4 & 12 \end{pmatrix}$, $\#250\ \begin{pmatrix} 4 & 0 \\ 0 & 16 \end{pmatrix}$, $\#251\ \begin{pmatrix} 6 & 2 \\ 2 & 8 \end{pmatrix}$, $\#252\ \begin{pmatrix} 8 & -4 \\ -4 & 8 \end{pmatrix}$, $\#253\ \begin{pmatrix} 6 & 0 \\ 0 & 12 \end{pmatrix}$, $\#254\ \begin{pmatrix} 12 & 0 \\ 0 & 12 \end{pmatrix}$, $\#255\ \begin{pmatrix} 12 & 2 \\ 2 & 12 \end{pmatrix}$, $\#256\ \begin{pmatrix} 12 & -6 \\ -6 & 10 \end{pmatrix}$, $\#257\ \begin{pmatrix} 4 & 0 \\ 0 & 20 \end{pmatrix}$, $\#258\ \begin{pmatrix} 8 & 0 \\ 0 & 8 \end{pmatrix}$, $\#259\ \begin{pmatrix} 10 & 2 \\ 2 & 10 \end{pmatrix}$, $\#260\ \begin{pmatrix} 12 & -6 \\ -6 & 12 \end{pmatrix}$, $\#261\ \begin{pmatrix} 12 & 0 \\ 0 & 12 \end{pmatrix}$, $\#262\ \begin{pmatrix} 10 & 0 \\ 0 & 10 \end{pmatrix}$, $\#263\ \begin{pmatrix} 6 & 0 \\ 0 & 18 \end{pmatrix}$, $\#264\ \begin{pmatrix} 20 & -10 \\ -10 & 20 \end{pmatrix}$, $\#265\ \begin{pmatrix} 12 & -6 \\ -6 & 18 \end{pmatrix}$, $\#266\ \begin{pmatrix} 8 & -4 \\ -4 & 20 \end{pmatrix}$, $\#267\ \begin{pmatrix} 24 & -12 \\ -12 & 24 \end{pmatrix}$, $\#268\ \begin{pmatrix} 24 & -12 \\ -12 & 24 \end{pmatrix}$, $\#269\ \begin{pmatrix} 8 & 0 \\ 0 & 16 \end{pmatrix}$, $\#270\ \begin{pmatrix} 12 & 0 \\ 0 & 24 \end{pmatrix}$, $\#271\ \begin{pmatrix} 12 & 0 \\ 0 & 12 \end{pmatrix}$, $\#272\ \begin{pmatrix} 20 & 0 \\ 0 & 20 \end{pmatrix}$, $\#273\ (\ 4\ )$, $\#274\ (\ 6\ )$, $\#275\ (\ 8\ )$, $\#276\ (\ 12\ )$, $\#277\ (\ 10\ )$, $\#278\ (\ 12\ )$, $\#279\ (\ 20\ )$, $\#280\ (\ 24\ )$, $\#281\ (\ 16\ )$, $\#282\ (\ 18\ )$, $\#283\ (\ 28\ )$, $\#284\ (\ 40\ )$, $\#285\ (\ 60\ )$, $\#286\ (\ 42\ )$, $\#287\ (\ 36\ )$, $\#288\ (\ 24\ )$, $\#289\ (\ 72\ )$, $\#290\ ()$.
